# Supplementary material for: Agglomerative Attention
Source: arXiv:1907.06607 ancillary file (2019-07-15)
Supplement: Supplementary file 1 [file SI_Notebook_A._Size_Benchmarks.pdf]

# SI Notebook A. Size Benchmarks

July 15, 2019

## 1 Introduction

This notebook performs simple scaling analysis on agglomerative attention layers. To isolate the effects of algorithmic complexity and avoid the complexities of dealing with load balancing and GPU memory limitations, this notebook runs on a single CPU core.

### 1.1 keras\_transformer Installation

This notebook requires a modified version of [keras\\_transformer](#), which was developed by [Kirill Mavreshko](#). The modified version can be installed from source as follows:

```
git clone https://github.com/klarh/keras-transformer
pip install -e ./keras-transformer
```

```
In [1]: import os
        # don't allow tensorflow to find any GPUs that are present
        os.environ['CUDA_VISIBLE_DEVICES'] = ''
        import numpy as np
        import keras
        import keras.backend as K
        import matplotlib, matplotlib.pyplot as pp
        import sys
        import tensorflow as tf
        import timeit
        import collections
        import itertools
        import tqdm
        import gc

        import keras_transformer, keras_transformer.attention

        # don't allow tensorflow to use CPU parallelism
        tf_config = tf.ConfigProto(
            intra_op_parallelism_threads=1,
            inter_op_parallelism_threads=1,
        )
        tf_config.gpu_options.allow_growth = True
        tf_config.graph_options.optimizer_options.global_jit_level = tf.OptimizerOptions.OFF
```

```

session = tf.Session(config=tf_config)
K.set_session(session)

```

Using TensorFlow backend.

```

In [2]: def make_model(seq_len, input_dim=512, attn_heads=4,
                    agglomerative=False, use_masking=True):
    inputs = keras.layers.Input(shape=(seq_len, input_dim))
    if agglomerative:
        attn = keras_transformer.attention.MultiHeadAgglomerativeSelfAttention(
            num_heads=attn_heads, use_masking=use_masking)(inputs)
    else:
        attn = keras_transformer.attention.MultiHeadSelfAttention(
            num_heads=attn_heads, use_masking=use_masking)(inputs)

    result = K.function([inputs], [attn])
    return inputs, result

In [3]: timings = collections.defaultdict(list)
seq_lens = np.linspace(2048, 16, 16).astype(np.uint32)//16*16
seq_lens = list(reversed(np.unique(seq_lens)))
aggloms = [False, True]
masks = [False, True]
replicas = list(range(5))
call_number = 3

INPUT_DIM = 512
NUM_HEADS = 8
BATCH_SIZE = 32

def tqdm_auto(*args):
    total = np.product([len(v) for v in args])

    result = itertools.product(*args)
    result = tqdm.tqdm_notebook(result, total=total)
    return result

iterations = tqdm_auto(seq_lens, aggloms, masks, replicas)

for (seq_len, agglomerative, mask, _) in iterations:
    key = (seq_len, agglomerative, mask)
    (inp_var, m) = make_model(
        seq_len, INPUT_DIM, NUM_HEADS, agglomerative, mask)
    inp = np.random.normal(size=(BATCH_SIZE, seq_len, INPUT_DIM))

    t = timeit.timeit('m([inp])', number=call_number, globals=globals())
    K.clear_session()

```

```

gc.collect()
timings[key].append(t/call_number)

HBox(children=(IntProgress(value=0, max=320), HTML(value='')))

WARNING:tensorflow:From /usr/lib/python3.7/site-packages/tensorflow/python/framework/op_def_library.py:266:
Instructions for updating:
Colocations handled automatically by placer.

```

```

In [4]: colors = pp.rcParams['axes.prop_cycle'].by_key()['color']

for (agglom, color) in zip(aggloms, colors):
    for mask in masks:
        xs, ys, sigs = [], [], []
        for seq_len in seq_lens:
            key = (seq_len, agglom, mask)
            mu, error = np.mean(timings[key]), np.std(timings[key])

            error /= np.sqrt(len(timings[key]))

            xs.append(seq_len)
            ys.append(mu)
            sigs.append(error)

        ys = np.array(ys)

        label = 'agg.' if agglom else 'full'
        if mask:
            label = label + ', masked'

        linestyle = '-' if mask else '--'
        # hide error bars for final version of figure since they are so small
        pp.fill_between(xs, ys - sigs, ys + sigs, color='gray', alpha=.5)
        pp.plot(xs, ys, label=label, color=color, linestyle=linestyle)

pp.xlabel('Sequence length')
pp.ylabel('Runtime / s')
pp.legend()
pp.savefig('../media/sequence_length_runtime.pdf')

```

```

/usr/lib/python3.7/site-packages/matplotlib/figure.py:2369: UserWarning: This figure includes
warnings.warn("This figure includes Axes that are not compatible ")

```

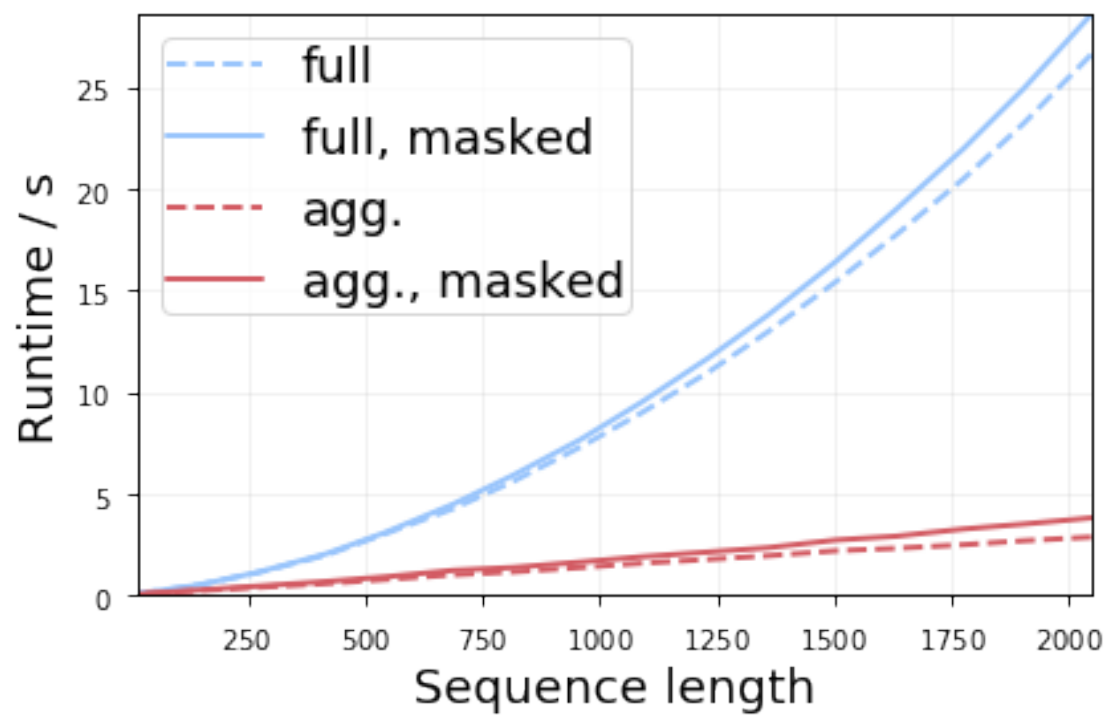

In [ ]:
